# Supplementary material for: Search for $C\!P$ violation in $\Lambda^0_b \to p K^-$ and $\Lambda^0_b \to p \pi^-$ decays
Source: arXiv:1807.06544 source file (2018-11-09)
Supplement: Supplementary file 1 [file supplementary-app.tex]

\clearpage

\section{Supplementary material for LHCb-PAPER-2018-025}
\label{sec:Supplementary-App}

This appendix contains supplementary material that will posted
on the public cds record but will not appear in the paper.

%Please leave the above sentence in your draft for first and
%second circulation and replace what follows by your actual supplementary material.
%For more information about other types of supplementary material, see Section~\ref{sec:Supplementary}. Plots and tables that follow should be well described, either with captions or with additional explanatory text.

\begin{figure}[!tbp]
\includegraphics[width=0.49\textwidth]{selPK_Lb2PPI}
\includegraphics[width=0.49\textwidth]{selPK_Lb2PIP}\\
\includegraphics[width=0.49\textwidth]{selPK_Bd2KPI}
\includegraphics[width=0.49\textwidth]{selPK_Bd2PIK}\\
\includegraphics[width=0.49\textwidth]{selPK_Bd2PIPI}
\includegraphics[width=0.49\textwidth]{selPK_Bs2KK}\\
\vspace{-0.5cm}
\caption{Invariant-mass distributions: (top left) $m_{\proton \pim}$, (top right) $m_{\antiproton \pip}$, (middle left) $m_{\Kp\pim}$, (middle right) $m_{\pip\Km}$, (bottom left) $m_{\pip\pim}$ and (bottom right) $m_{\Kp\Km}$ for the \SpK selection. The results of the fits are superimposed.}
\label{fig:FitProjSelPK}
\end{figure}

\begin{figure}[!tbp]
\includegraphics[width=0.49\textwidth]{selPPI_Lb2PK}
\includegraphics[width=0.49\textwidth]{selPPI_Lb2KP}\\
\includegraphics[width=0.49\textwidth]{selPPI_Bd2KPI}
\includegraphics[width=0.49\textwidth]{selPPI_Bd2PIK}\\
\includegraphics[width=0.49\textwidth]{selPPI_Bd2PIPI}
\includegraphics[width=0.49\textwidth]{selPPI_Bs2KK}\\
\vspace{-0.5cm}
\caption{Invariant-mass distributions: (top left) $m_{\proton \Km}$, (top right) $m_{\antiproton \Kp}$, (middle left) $m_{\Kp\pim}$, (middle right) $m_{\pip\Km}$, (bottom left) $m_{\pip\pim}$ and (bottom right) $m_{\Kp\Km}$ for the \Sppi selection. The results of the fits are superimposed.}
\label{fig:FitProjSelPPI}
\end{figure}

\clearpage
